# Supplementary material for: Stationary shapes of axisymmetric vesicles beyond lowest-energy configurations
Source: arXiv:2311.14193 ancillary file (2023-11-23)
Supplement: Supplementary file 1 [file Vesicle_Shapes_Supplementary_Material_Arxiv.pdf]

# Supplementary Material - Stationary shapes of axisymmetric vesicles beyond lowest-energy configurations

Rodrigo B. Reboucas, Hammad A. Faizi, Michael J. Miksis and Petia M. Vlahovska

## 1 Notes on differential geometry

Let a surface be defined by $\mathbf{x} = \mathbf{x}(u, v)$ in rectangular coordinates, where $u, v$ surface coordinates. Figure 1 shows surface vectors at point $P$, where the tangent vectors $(\mathbf{x}_u, \mathbf{x}_v)$ span a tangent plane locally and $\mathbf{n}$ is the normal vector given by

$$\mathbf{n} = \frac{\mathbf{x}_u \times \mathbf{x}_v}{|\mathbf{x}_u \times \mathbf{x}_v|} = \frac{\mathbf{x}_u \times \mathbf{x}_v}{\sqrt{EG - F^2}} \tag{1.1}$$

where the direction of the normal depends on the labelling of the coordinate curves. Here, $E$, $F$, and $G$ are the coefficients of the first fundamental form in differential geometry [1]

$$E = \mathbf{x}_u \cdot \mathbf{x}_u\,, \quad F = \mathbf{x}_u \cdot \mathbf{x}_v\,, \quad G = \mathbf{x}_v \cdot \mathbf{x}_v\,, \tag{1.2}$$

and hence the differential element of area can be expressed as

$$dA = \sqrt{EG - F^2} du\, dv\,, \tag{1.3}$$

where $W = \sqrt{EG - F^2}$ defines a local metric on the surface. The general equation for the mean curvature and Gaussian curvatures are

$$\mathrm{H} = \frac{1}{2}\frac{EN - 2FM + GL}{W^2} = \frac{1}{2}(c_1 + c_2)\,, \tag{1.4}$$

and

$$K = \frac{LN - M^2}{W^2} = c_1\, c_2\,, \tag{1.5}$$

where $c_1$ and $c_2$ are the principal curvatures, and

$$L = \mathbf{x}_{uu} \cdot \mathbf{n}\,, \quad M = \mathbf{x}_{uv} \cdot \mathbf{n}\,, \quad \bar{N} = \mathbf{x}_{vv} \cdot \mathbf{n}\,, \tag{1.6}$$

are the coefficients of the second fundamental form. In the case where parametric lines coincide with lines of curvature, the principal curvatures in (1.4) reduce to

$$c_1 = \frac{L}{E}\,, \quad c_2 = \frac{N}{G}\,, \tag{1.7}$$

since $F = M = 0$.

It is useful to define the Laplace-Beltrami operator,

$$\Delta_b f = \frac{1}{W}\left(\left(\frac{Ef_v - Ff_u}{W}\right)_v + \left(\frac{Gf_u - Ff_v}{W}\right)_u\right)\,, \tag{1.8}$$

where $f$ is an arbitrary function. For axisymmetric geometries, $F = 0$ and the $v$-derivatives are set to zero, and hence Eq. (1.8) reduces to

$$\Delta_b f = \frac{1}{W}\left(\frac{G f_u}{W}\right)_u . \tag{1.9}$$

In the general literature on vesicle shapes [2], the metric coefficient $g$ is defined as the determinant of the metric tensor $g_{ij} \equiv \mathbf{x}_i \cdot \mathbf{x}_j$, for $i, j = 1, 2$ such that

$$g_{ij} = \begin{pmatrix} E & F \\ F & G \end{pmatrix} , \tag{1.10}$$

and the curvature tensor $h_{ij} \equiv (\partial_i \partial_j \mathbf{x}) \cdot \mathbf{n}$ is

$$h_{ij} = \begin{pmatrix} L & M \\ M & N \end{pmatrix} . \tag{1.11}$$

Accordingly, the mean curvature in Eq.(1.4) is equivalent to $\mathrm{H} \equiv tr(h^i_j)/2$ where $h^i_j \equiv g^{ik} h_{kj}$ and $g^{ik}$ are the components of the inverse of the metric tensor (1.10), and hence

$$h^i_j = \begin{pmatrix} L/E & 0 \\ 0 & N/G \end{pmatrix} , \tag{1.12}$$

in agreement with Eq. (1.7).

An important distinction between the notation used in standard differential geometry for the mean curvature, H, and the notation used in the literature on vesicle shape equations, $H$, is the sign-convention where $H = -\mathrm{H}$. This convention is adopted so that in the limit of a spherical shape, the mean curvature, $H$, is positive using the standard spherical coordinates notation (i.e., $u = \theta$, and $v = \phi$); see, for instance, the discussion below Eq. (2.9) in Ref. [2].

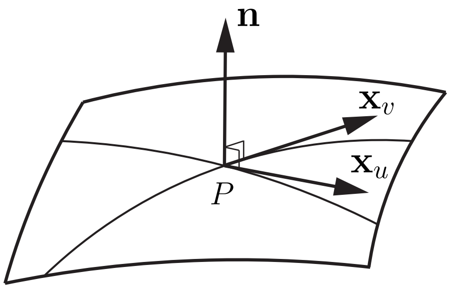


Figure 1: Local representation of the tangent vectors $(\mathbf{x}_u, \mathbf{x}_v)$ at a point $P$ on a surface represented by $\mathbf{x} = \mathbf{x}(u, v)$; outward-pointing normal vector, $\mathbf{n}$, as indicated.

### 1.1 Arclength parametrization

The position vector of a point on a axisymmetric surface parameterized by arclength, as shown in Fig.1(b) in the main text, where $u = s$ and $v = \phi$ is

$$\mathbf{x}(s, \phi) = \{r(s)\cos\phi,\ r(s)\sin\phi,\ z(s)\} , \tag{1.13}$$

where $s$ is the arclength and $\phi$ is the azimuthal angle. Using (1.13) in Eq.(1.1) yields the surface normal

$$\mathbf{n}(s, \phi) = \{-z_s \cos\phi, -z_s \sin\phi, r_s\} . \tag{1.14}$$

Using relations (1.13) and (1.14) the coefficients of the first and second fundamental forms reduce to

$$E = 1\,, \quad F = 0\,, \quad G = r^2 \tag{1.15}$$

and

$$L = r_s z_{ss} - z_s r_{ss}\,, \quad M = 0\,, \quad N = r\, z_s\,. \tag{1.16}$$

Using Eqs. (1.7) the principal curvatures are given by

$$c_1 = r_s z_{ss} - z_s r_{ss}\,, \tag{1.17}$$

and

$$c_2 = \frac{z_s}{r}\,. \tag{1.18}$$

Thus, the mean curvature is completely defined (i.e., $\mathrm{H} = -H$), aside from a minus sign depending on the choice of notation. In the arclength parametrization, the Laplace-Beltrami of operator given by (1.9) reduces to

$$\Delta_b f = \frac{1}{r}\left(r f_s\right)_s\,. \tag{1.19}$$

In the tilt-angle formulation, $r_s = \cos\psi$ and $z_s = -\sin\psi$, the principal curvatures are

$$c_1 = -\psi_s\,, \tag{1.20}$$

and

$$c_2 = -\frac{\sin\psi}{r}\,. \tag{1.21}$$

## 1.2 Force balance approach

A complementary approach to deriving the general shape equations following a force balance at the interface is presented. The elastic traction per unit area acting on the membrane can be obtained from

$$\mathbf{f}_m = \frac{\delta^{(1)} E_b}{\delta \mathbf{x}} + \frac{\delta^{(1)} E_\Sigma}{\delta \mathbf{x}}\,, \tag{1.22}$$

such that

$$\mathbf{f}_m = \left[-2\kappa\Delta_b H - 4\kappa H(H^2 - K) + 2H\Sigma\right]\mathbf{n} - \nabla_s\Sigma\,, \tag{1.23}$$

using the results from Appendix A in the main text and setting $\mathrm{H} = -H$. The hydrostatic stress is discontinuous across the interface and is balanced by internal membrane stresses,

$$\mathbf{n}\cdot\left[\mathbf{T}^h_{ex} - \mathbf{T}^h_{in}\right] = \mathbf{f}_m\,, \tag{1.24}$$

where $T^h_{ij,k} = -p_k\delta_{ij}$ is the second-order, hydrostatic stress tensor and the subscript $k = ex\,, in$ indicates the exterior and interior regions of the closed vesicle, respectively. Hence,

$$-P\mathbf{n} = \mathbf{f}_m\,, \tag{1.25}$$

where $P = p_{ex} - p_{in}$, following the definition of pressure difference used in Eq. (**??**). Combining Eqs. (1.25) and (1.23) yields the force balance in the normal direction,

$$2\kappa\Delta_b H + 4\kappa H(H^2 - K) - 2H\Sigma - P = 0 \tag{1.26}$$

in agreement with Eq. (8) in the main text.

## 2 Hamilton's Principle of Stationary Action

In this section we present a derivation of Hamilton's principle of stationary action following [3] to complement the discussion on the tilt-angle formulation for stationary shapes presented in Appendix C in the main text. Hamilton's principle of stationary action is typically associated with the minimum of an action functional defined as

$$S = \int_{t_i}^{t_f} \mathcal{L}(\mathbf{q}(t), \dot{\mathbf{q}}(t), t) dt \,, \tag{2.1}$$

where $\mathcal{L}$ is the Lagrangian of a system in a configurational space spanned by $n$ generalized coordinates $\mathbf{q}$ and velocities $\dot{\mathbf{q}}$. Let the scalar action $S$ represent the extremum path between initial and final states of a system at two different times $t_i$ and $t_f$, respectively. Taking the variation of S by sampling through a family of neighbouring paths defined at $t_i \to t_i + \Delta t_i$, $t_f \to t_f + \Delta t_f$, and $q_j(t) \to q_j(t) + \delta q_j(t)$, where $\delta$ represents an infinitesimal virtual displacement, yields the incremental change in the action

$$\delta S = \int_{t_i}^{t_f} \sum_j \left( \frac{\partial \mathcal{L}}{\partial q_j} \delta q_j + \frac{\partial \mathcal{L}}{\partial \dot{q}_j} \delta \dot{q}_j \right) dt + \left[ \mathcal{L} \Delta t \right]_{t_i}^{t_f} \,, \tag{2.2}$$

where $j = 1, \ldots, n$ spans the space of generalized coordinates and velocities. Integrating by parts the second term in the sum of Eq. (2.2), results in

$$\delta S = \int_{t_i}^{t_f} \sum_j \left( \frac{\partial \mathcal{L}}{\partial q_j} - \frac{d}{ds} \frac{\partial \mathcal{L}}{\partial \dot{q}_j} \right) \delta q_j \, dt + \left[ \mathcal{L} \Delta t - \sum_j \frac{\partial \mathcal{L}}{\partial \dot{q}_j} \delta q_j \right]_{t_i}^{t_f} \,. \tag{2.3}$$

Equation (2.3) includes the variation of the Lagrangian along the path, and additional variations at the endpoints including the effect of increments in time between neighbouring paths.

The stationary principle in Lagrangian mechanics is centered on the determination of extremum paths undertaken by a system between two fixed locations in configurational space at two different times (e.g., $\mathbf{q}_j(t_i)$ and $\mathbf{q}_j(t_f)$). The end coordinate points are fixed and hence $\delta q_j(t_i) = \delta q_j(t_f) = 0$ and $\Delta t_i = \Delta t_f = 0$; in this limit, Eq.(2.3) simplifies to

$$\delta \tilde{S} = \int_{t_i}^{t_f} \sum_j \left( \frac{\partial \mathcal{L}}{\partial q_j} - \frac{d}{ds} \frac{\partial \mathcal{L}}{\partial \dot{q}_j} \right) \delta q_j \, dt \,, \tag{2.4}$$

where, for independent variations of the generalized coordinates, the term in parenthesis vanishes yielding a stationary path (i.e., $\delta \tilde{S} = 0$) along which the system evolves in time according to the Euler-Lagrange equations.

The stationary principle in Hamiltonian mechanics, involves the general variation of the Lagrangian functional as shown in (2.3), where the relative action between two paths is taken at different initial and final locations at different initial and final times. The integral term in (2.3) vanishes yielding a set Euler-Lagrange equations for the system, and the remaining term contains endpoint contributions to the variation. Let the total variation at each endpoint be defined as

$$\Delta q_j = \delta q_j + \dot{q}_j \, \Delta t \,; \tag{2.5}$$

inserting (2.5) into the second term on the right-hand-side of Eq.(2.3) results in

$$\delta S = \left[ \sum_j \frac{\partial \mathcal{L}}{\partial \dot{q}_j} \Delta q_i - \mathcal{H} \Delta t \right]_{t_i}^{t_f} \,, \tag{2.6}$$

where

$$\mathcal{H} \equiv -\mathcal{L} + \sum_j \frac{\partial \mathcal{L}}{\partial \dot{q}_j} \dot{q}_i \,, \tag{2.7}$$

is the Hamiltonian of the system, and Eq.(2.7) represents Hamilton's principle of least action.

# 3 Stationary shapes of GUVs

All the stationary shapes marked as (i)-(j) in Fig. 3 in the main text are shown here for completeness. The parameter values of each shape are listed in Table 1 in the main text.

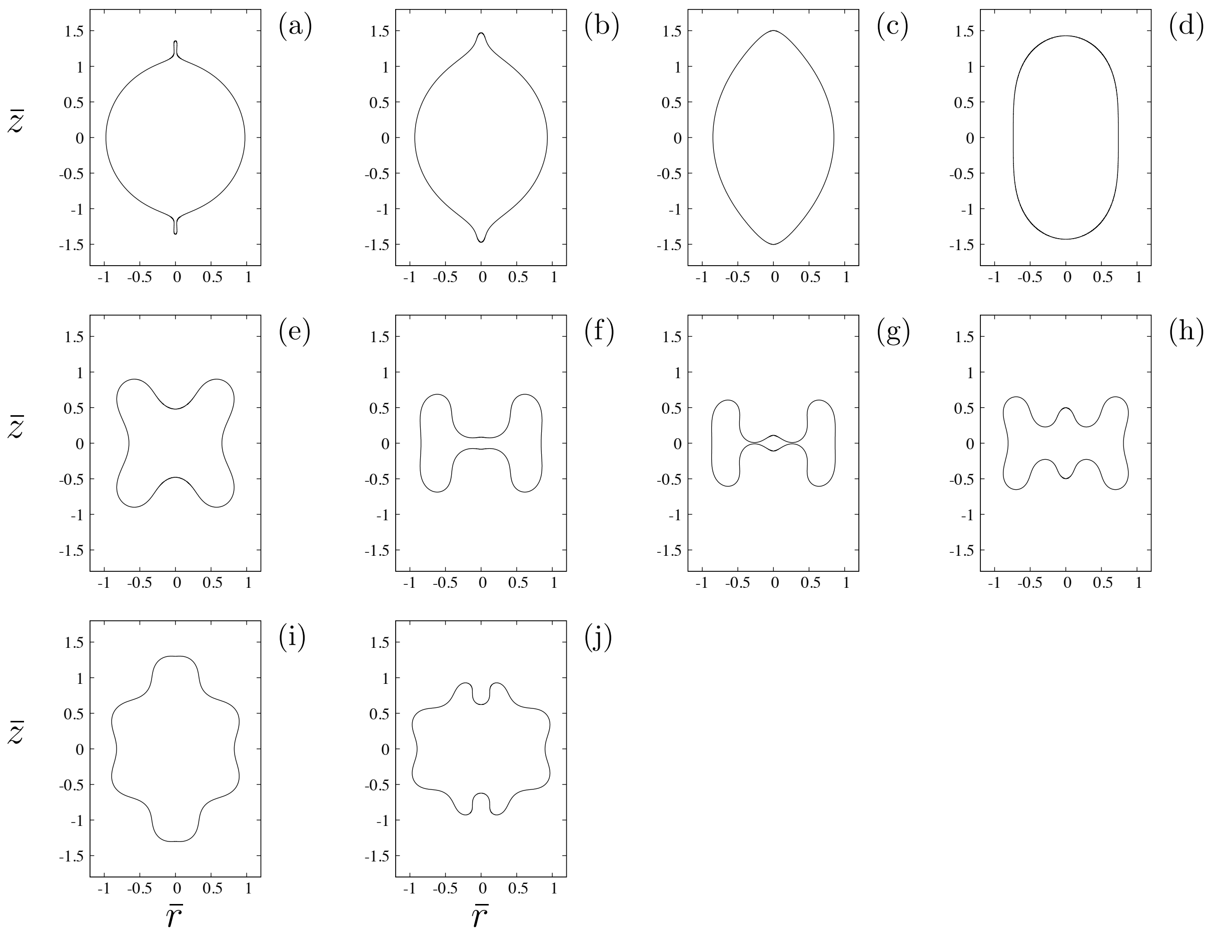


Figure 2: Vesicle shapes for a fixed $\bar{A} = 1$, and $\bar{L} = 3.62$; as indicated by the labels in Fig. ??; additional data on relevant parameters is listed in Table 1 of the main text.

# References


[1] Dirk Jan Struik. *Lectures on classical differential geometry.* Courier Corporation, 1961.

[2] Udo Seifert. Configurations of fluid membranes and vesicles. *Advances in Physics*, 46(1):13–137, 1997.

[3] Douglas Cline. *Variational principles in classical mechanics.* University of Rochester River Campus Librarie, 2017.
